# Supplementary material for: Axion dark matter search with a photonic bandgap cavity haloscope and dielectric tuning rod over 10.25-10.45 GHz
Source: arXiv:2608.07718 source file (2026-08-07)
Supplement: Supplementary file 1 [file Supplementary_Material.tex]

This document provides additional details pertaining to the experiment described in the main text. Namely, the full wiring diagram of the experimental setup in our dilution refrigerator, the temperature of the piezoelectric motor during a cooldown to prevent freezing on the motor gears, and a characterization of mechanically induced cavity mode broadening. 
\subsection{Piezo Heating During Cooldown}
\indent From the main body, we thermally isolate the piezoelectric motor from the dilution refrigerator during a cooldown to prevent freezing. Even a few degrees difference has shown to be sufficient.
\begin{figure}[htbp]
\centering
\includegraphics[width=\columnwidth]{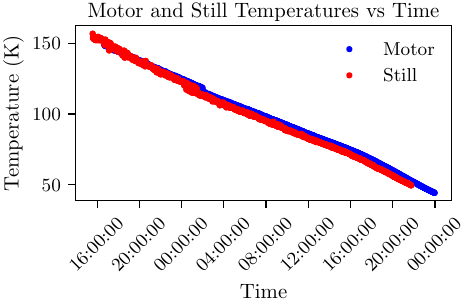}
 \caption[Motor Temperature During Cooldown]{Temperature of the piezoelectric motor during a cooldown compared to the still plate of the refrigerator, where the motor is heat sunk to. Even a few degrees of difference between the motor and the refrigerator has been sufficient to get consistent use of the motor.}
 \label{fig:Motor Temperatures}
\end{figure}
\FloatBarrier
\subsection{Fridge Diagram}
\begin{figure}[htbp]
\centering
\includegraphics[width=\columnwidth, height=0.6\textheight, keepaspectratio]{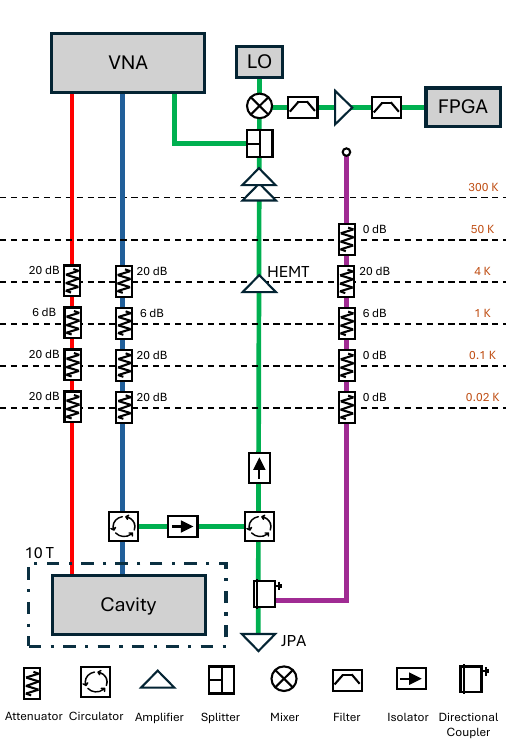}
  \caption[Fridge Schematic]{Experimental setup inside the dilution refrigerator. Cavity parameters are measured either in transmission or reflection with a common output line. The cavity sits in the center of the magnet bore (dashed box), with the magnet heat sunk to the $4$ K stage of the refrigerator. While a JPA was installed it was not used due to unstable gain with the magnet ramped. In its place the HEMT amplifier was the first stage amplifier.}
  \label{fig:fridge wiring}
\end{figure}
\FloatBarrier
\subsection{Cavity Broadening}
\input{Amplitude_oscillations}
